# Supplementary material for: On the Robustness of Fairness Practices: A Causal Framework for Systematic Evaluation
Source: arXiv:2601.03621 source file (2026-01-07)
Supplement: Supplementary file 1 [file Appendix.tex]

\appendix
\section{Appendix}
\label{sec:appendix}

\begin{algorithm}[!bht]
\scriptsize
\DontPrintSemicolon
    \KwIn{Dataset $\mathcal{A}$, ML algorithm $\mathcal{M}$, Default HP $h\textsubscript{0}$, 
    Non-sensitive attributes $\mathcal{NP}$, Sensitive attributes $\mathcal{P}$, type of analysis $\tau$,
    Feature selection method $f\_s$, the step size $stp\_size$, HP constraints $\mathcal{S}$, Max. HP search $N$,
    and Timeout $\mathcal{T}$.
    }
    $\mathcal{G}$, $edges\_list$ $\gets$ \texttt{CausalDiscovery}($\mathcal{A}$) \Comment{Causal Discovery} \\
    $\mathcal{W^G}$ $\gets$ \texttt{Stan}($\mathcal{G}$, $edges\_list$) \Comment{Causal Inference} \\
    $\mathcal{A\textsubscript{0}}$ $\gets$ \texttt{Generate}($\mathcal{G}$, $\mathcal{W^G}$)\\
    $EOD\textsubscript{0}$, $Acc\textsubscript{0}$ $\gets$ \texttt{Train}($\mathcal{M}$, $h\textsubscript{0}$, $\mathcal{A\textsubscript{0}}, \mathcal{P}$)\\
    % $EOD_{max}$ $\gets$  $EOD\textsubscript{0}$\\

    $Found$, $t$, $t_0$ $i$, $\mathcal{G}_0$, $\mathcal{W^G_\textsubscript{0}}$ $\gets$ \texttt{False}, 0, 0, \texttt{time}(), $\mathcal{G}$, $\mathcal{W^G}$
    
    \While{$t \leq \mathcal{T}$}{
        $\mathcal{G\textsubscript{1}}$,  $\mathcal{W^G_\textsubscript{1}}$ $\gets$ \texttt{perturb}($\mathcal{G\textsubscript{0}}$, $\mathcal{W^G_\textsubscript{0}}$, $\mathcal{G}$, $\mathcal{W^G}$, $stp\_size$ )\\
        $\mathcal{A\textsubscript{1}}$ $\gets$ \texttt{Generate}($\mathcal{G\textsubscript{$1$}}$,  $\mathcal{W^G_\textsubscript{1}}$ )\\
        \If{$\tau$ == Drop\_Analysis}{
            $\mathcal{A\textsubscript{dropped}}$  $\gets$  \texttt{Drop}($\mathcal{A\textsubscript{1}}$, $\mathcal{P}$) \\
            $EOD_1$, $Acc\textsubscript{1}$ $\gets$ \texttt{Train}($\mathcal{M}$, $h_0$, $\mathcal{A\textsubscript{dropped}}$, $\mathcal{P}$)\\
            \If{$EOD_0$ > $EOD_1$}{
                 $\mathcal{G\textsubscript{$\mathcal{P}$}}$ $\gets$ $\mathcal{G\textsubscript{1}}$

                $Found$ $\gets$ \texttt{True}
            }
        }
        \If{$\tau$ == featureSelection\_Analysis}{
            // {\color{black}f\_s: \texttt{Random}, \texttt{Kbest}, \texttt{Fpr}, or \texttt{Percentile}}
                        
            $\mathcal{A\textsubscript{1}}$  $\gets$  \texttt{f\_s}($\mathcal{A\textsubscript{1}}$, $\mathcal{NP}$) \\

            $EOD_{1}$, $Acc_{1}$ $\gets$ \texttt{Train}($\mathcal{M}$, $h_0$,   $\mathcal{A\textsubscript{1}}$, $\mathcal{P}$)\\
            
            \If{$EOD_0$ > $EOD_1$}{
                 $\mathcal{G\textsubscript{$\mathcal{NP}$}}$ $\gets$ $\mathcal{G\textsubscript{1}}$

                $Found$ $\gets$ \texttt{True}
            }
        }   
        \If{$\tau$ == $\mathcal{HP}$\_Analysis}{
            
            \If{i == 0}{    
                \texttt{$HP_0$}, $EOD_0$  $\gets$ \texttt{HP\_Search}($\mathcal{M}$, $\mathcal{A\textsubscript{0}}$, $\mathcal{S}$, $h_0$, $N$)
                                
                $HP\_Imp_0$ $\gets$  \texttt{SHAP}$((HP_0, EOD_0))$          
            }
            
            \For{$h \in HP_0$}{
                $EOD\textsubscript{1}$, $Acc_{1}$ $\gets$ \texttt{Train}($\mathcal{M}$, $h$,  $\mathcal{A\textsubscript{1}}$, $\mathcal{P}$)\\
                $HP_1$.\texttt{add}($h$)
            }
           $HP\_Imp_1$ $\gets$ \texttt{SHAP}$((HP_1, EOD_1))$
           
           $distance$ $\gets$ \texttt{Distance}($HP\_Imp_0$,  $HP\_Imp_1$)
           
           \If{$distance$ > 2}{
                $\mathcal{G\textsubscript{$\mathcal{HP}$}}$ $\gets$  $\mathcal{G\textsubscript{$1$}}$

                $Found$ $\gets$ \texttt{True}
            }  
        }
        \If{{\it Found}}{
            Break
        }
        \If{\texttt{Interesting($\mathcal{G\textsubscript{1}}$,$\mathcal{G\textsubscript{0}}$)}}{
            $\mathcal{G\textsubscript{0}}$, $\mathcal{W^G_\textsubscript{0}}$ $\gets$ $\mathcal{G\textsubscript{1}}$, $\mathcal{W^G_\textsubscript{1}}$
        }
        $t$, $i$ $\gets$ \texttt{time}() - $t_0$, $i + 1$

    }
    return  $\mathcal{G_\textsubscript{0}}$, $\mathcal{G\textsubscript{$\mathcal{P}$}}$,  $\mathcal{G\textsubscript{$\mathcal{NP}$}}$, $\mathcal{A\textsubscript{1}}$,  $\mathcal{G\textsubscript{$\mathcal{HP}$}}$, $HP_1$
   
\caption{Causal Search}
\label{alg:algorithm1}
\end{algorithm}

In this section, we show the algorithm~\ref{alg:algorithm1} of our causal search approach described in the Approach section~\ref{sec:approach}.
Algorithm~\ref{alg:algorithm1} describes our approach to investigate the relationship between the causal graphs and common
practices in fairness training of ML models. We first use the input dataset to obtain the CPDAG representation (line 1). In line 2, we generate all possible equivalence DAGs from each CPDAG and infer a set of 1,000 causal graphs for each DAG with slightly different linear models (i.e.,
weights of linear functions connecting two features in the causal graph). We then use these graphs
to generate (i.i.d) samples the same size as the input datasets (line 3). To ensure the generated samples accurately reflect the real data distribution, we cluster the original input dataset into 100 clusters and calculate the average Euclidean distance between data points and their respective cluster centroids. For each generated sample, we calculate its distance to the nearest centroid and accept only those falling within the average distance calculated previously. This step ensures that accepted samples align with the true distribution of the real data, filtering out outliers and unrealistic data points. 
To assess the efficacy of our distance function in identifying in-distribution data samples, we performed a split of each dataset into training and testing sets. We computed the average distance criteria on the training set and evaluated the performance on the test set by measuring the True Positive Rate (TPR). To further understand the behavior of False Negative Rate (FNR), we generated a random uniform test set and applied the distance function to it. 
% The results of these tests are presented in the TPR and FNR columns of Table~\ref{table:dataset}. 
% The high TPR combined with a low FNR indicates the effectiveness of our distance function in evaluating the accuracy of our causal models. We then calculate the proportion of accepted samples for each causal graph as its success rate, reflecting the graph's ability to generate realistic data. Graphs demonstrating poor performance (low success rate) are excluded, effectively narrowing down the search space of possible causal structures. However, this validation step is bypassed when studying the robustness of practices under distribution shifts, as the focus then lies on understanding performance under different data distributions.

Once we identify a set of causal graphs, we run the search algorithm to validate whether a fairness practice (i.e., property)
holds true between two similar datasets. We note that the search depends on the type of property.
\emph{If the type of analysis is the effect of excluding sensitive attributes on fairness}, we simply exclude sensitive attributes from the generated data samples during training and measure the EOD bias (lines 9-14). \emph{If the type of analysis is the feature selection}, we use the following methods: \texttt{random} (i.e., exclude a subset of features at random up to 3 features during training), \texttt{SelectKBest}~\cite{KBest} (i.e., only include top $K$ features in training), \texttt{SelectFpr}~\cite{SelectFpr} (i.e., include features based on false positive rates), and \texttt{SelectPercentile}~\cite{SelectPercentile} (i.e., select top features based on their percentile scores) to select a subset of feature for training (lines 15-21). \emph{Finally, if the type of analysis is hyperproperty (HP)}, we adapted an evolutionary algorithm (\textsc{Parfait-ML}~\cite{10.1145/3510003.3510202}) to infer important HPs of the base graph. We start with the default HP and generate mutant seeds by mutating HP values. Each mutant's EOD metric is evaluated, and if it surpasses the lowest EOD seen so far, we include it in the next generation. We run this algorithm for a fixed time of $4$ hours to generate a large set of fairness-relevant HPs. We do the same analysis for the equivalence causal graphs and compare the important HPs to the base graph via SHAP~\cite{NIPS2017_7062}. If the rank of two HP variables from the top four HP variables has changed, we deem the DAG to violate the recommended hyperproperty configurations (lines 22-33).

We also list the identified equivalent causal graph by our search algorithm for Table\ref{tab:table_sens_nonsens} experiments. The protected attribute is circled with red color.

\begin{figure*}
 \begin{minipage}{0.24\textwidth}
   \centering
    \includegraphics[width=0.78\textwidth]{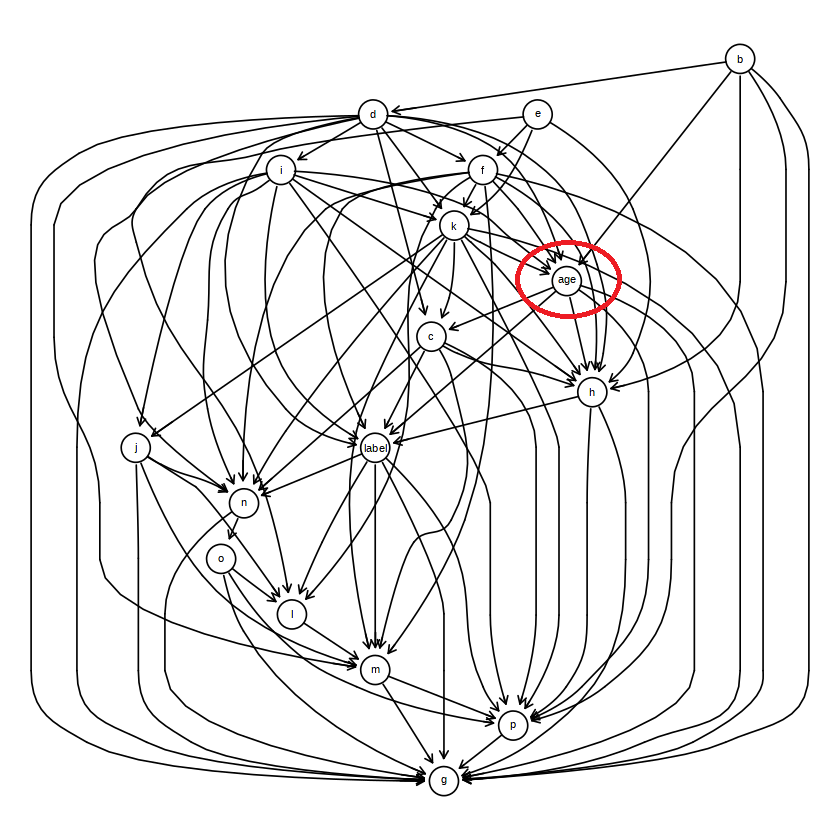}
    \includegraphics[width=0.795\textwidth]{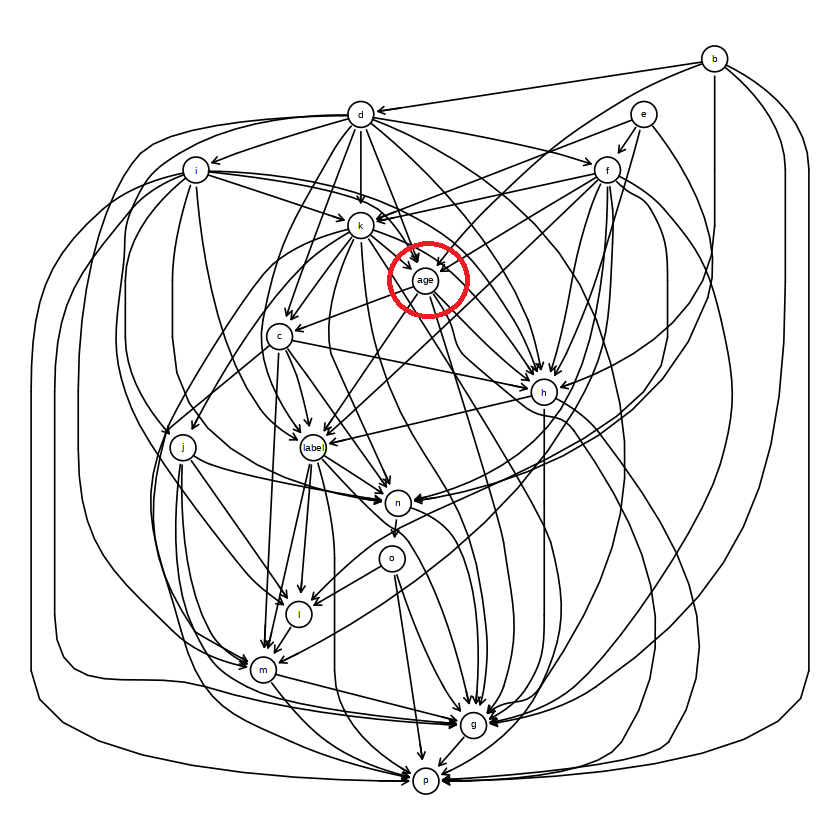}
    \captionsetup{font=small}
    \caption*{(a) Drop Sensitive.}
 \end{minipage}
 \begin{minipage}{0.24\textwidth}
   \centering
    \includegraphics[width=0.78\textwidth]{Figures/appendix/Bank_ges_DAG_4.png}
    \includegraphics[width=0.795\textwidth]{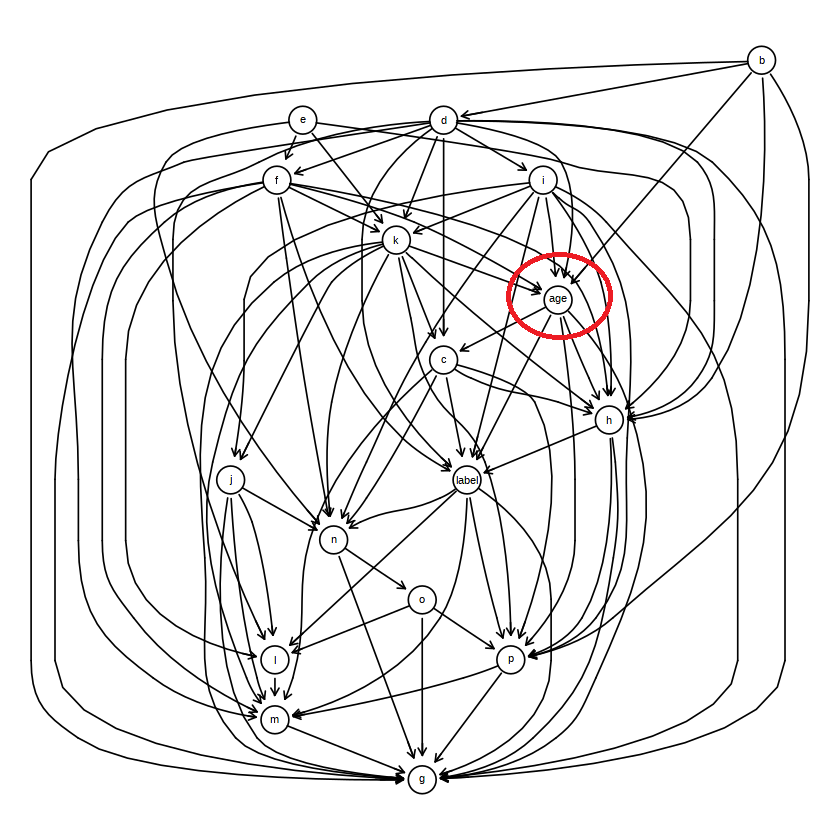}
    \captionsetup{font=small}
    \caption*{(b) SelectKbest.}
 \end{minipage}
  \begin{minipage}{0.24\textwidth}
   \centering
    \includegraphics[width=0.78\textwidth]{Figures/appendix/Bank_ges_DAG_3.png}
    \includegraphics[width=0.795\textwidth]{Figures/appendix/Bank_ges_DAG_3.png}
    \captionsetup{font=small}
    \caption*{(c) SelectFpr.}
 \end{minipage}
 \begin{minipage}{0.24\textwidth}
   \centering
    \includegraphics[width=0.78\textwidth]{Figures/appendix/Bank_ges_DAG_4.png}
    \includegraphics[width=0.795\textwidth]{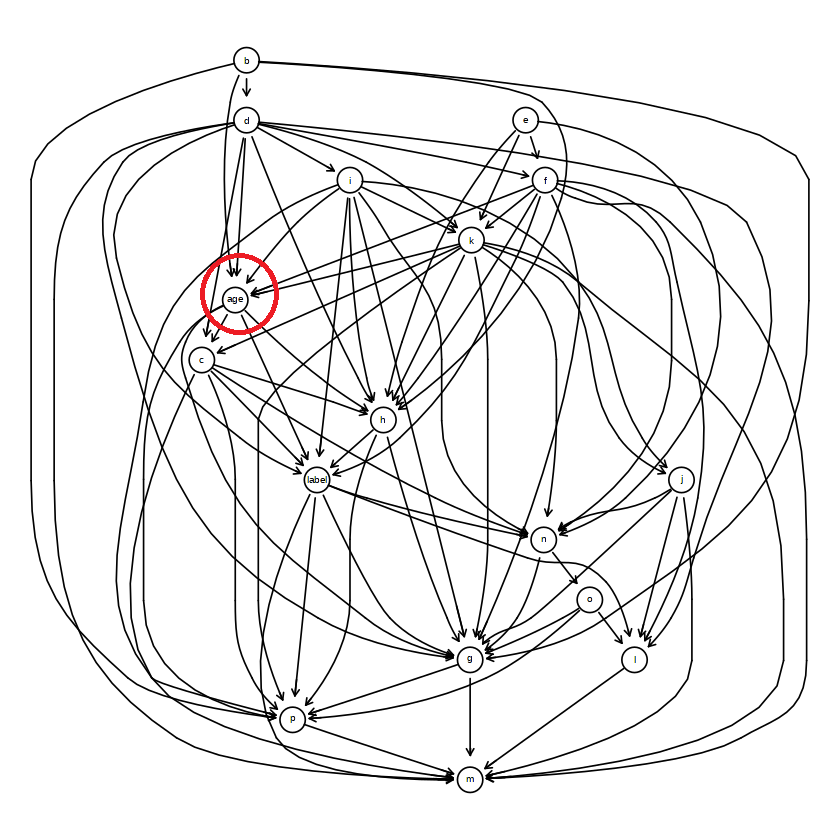}
    \captionsetup{font=small}
    \caption*{(d) SelectPercentile.}
 \end{minipage}
 \caption{Two (neighbor) causal graphs of Bank dataset with varying fairness for each feature selection practice.}
 \label{fig:causal-bank}
\end{figure*}

\begin{figure*}
  \begin{minipage}{0.3\textwidth}
   \centering
    \includegraphics[width=0.78\textwidth]{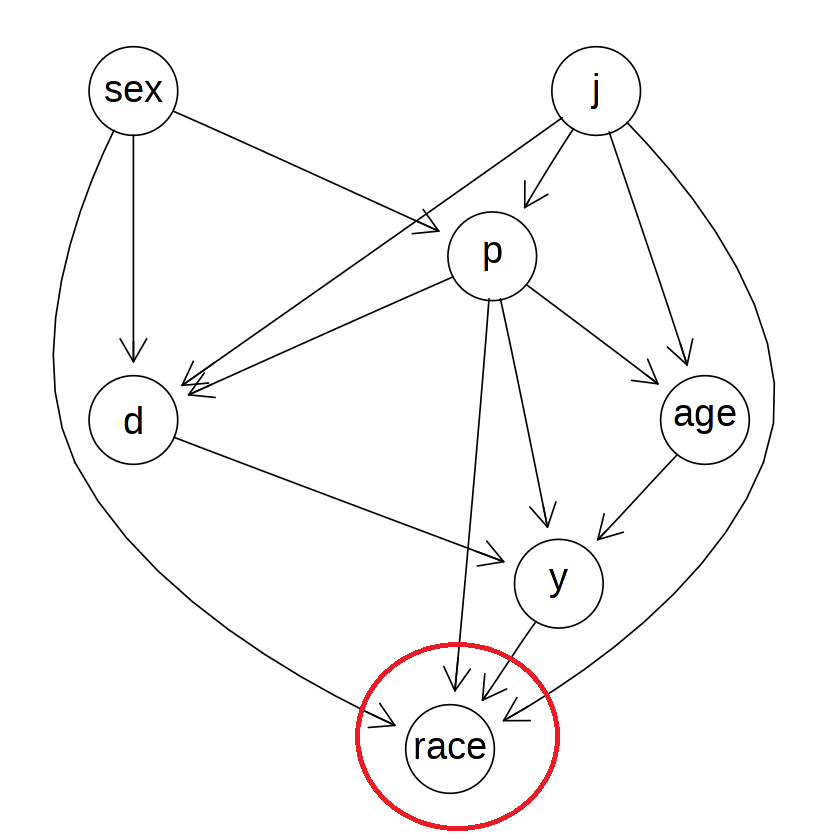}
    \includegraphics[width=0.795\textwidth]{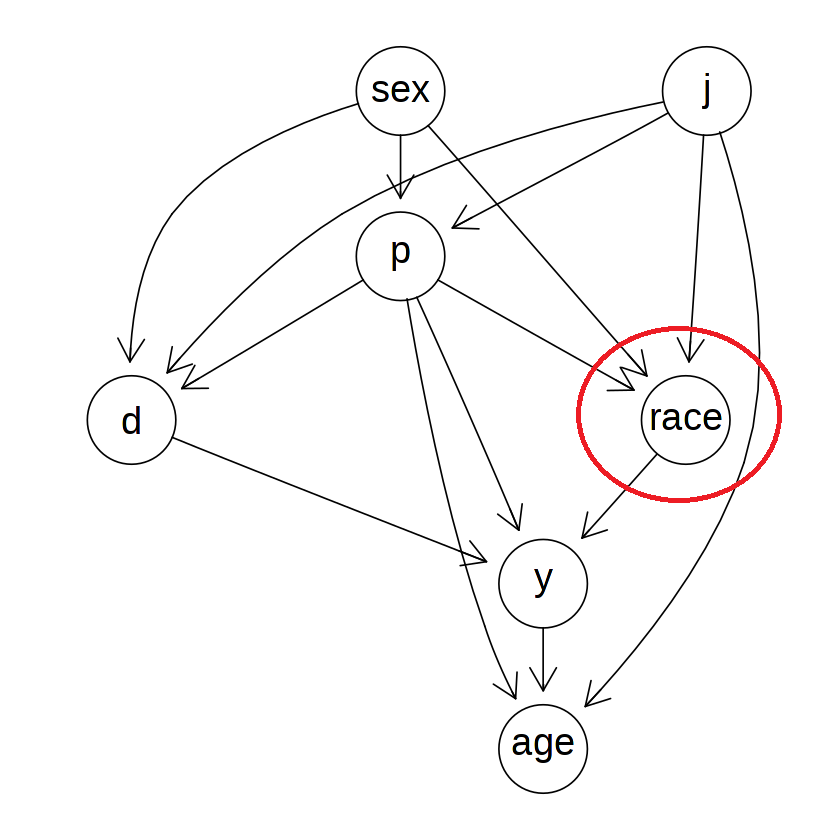}
    \captionsetup{font=small}
    \caption{COMPAS SelectKbest.}
    \label{fig:causal-compas}
 \end{minipage}
 \begin{minipage}{0.3\textwidth}
   \centering
    \includegraphics[width=0.78\textwidth]{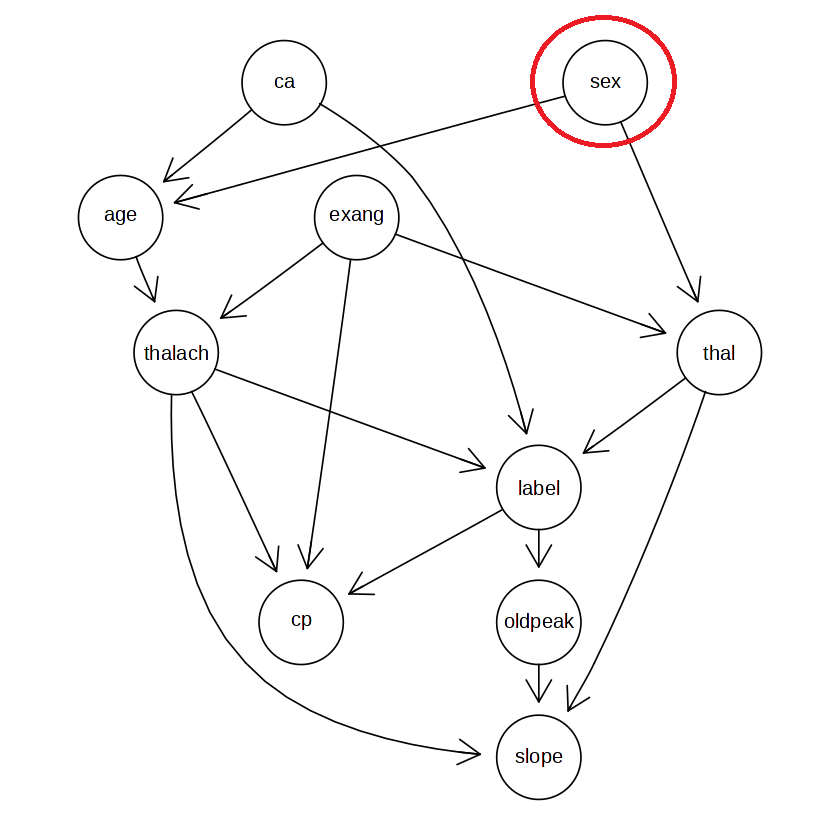}
    \includegraphics[width=0.795\textwidth]{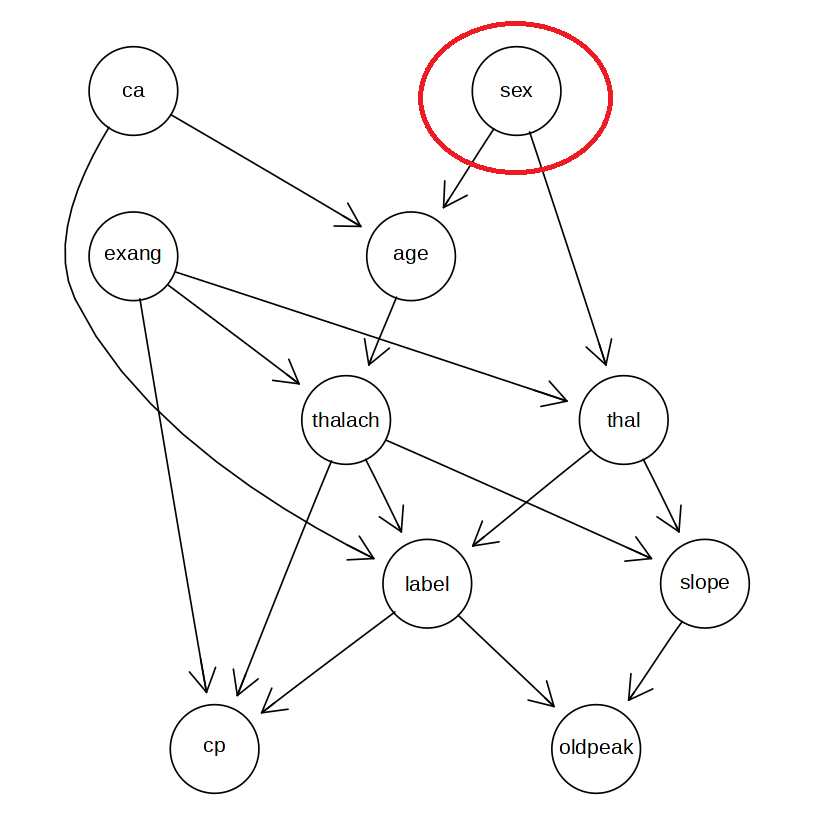}
    \captionsetup{font=small}
    \caption{Heart DropSens.}
    \label{fig:causal-heart-drop}
 \end{minipage}
 \begin{minipage}{0.3\textwidth}
   \centering
    \includegraphics[width=0.78\textwidth]{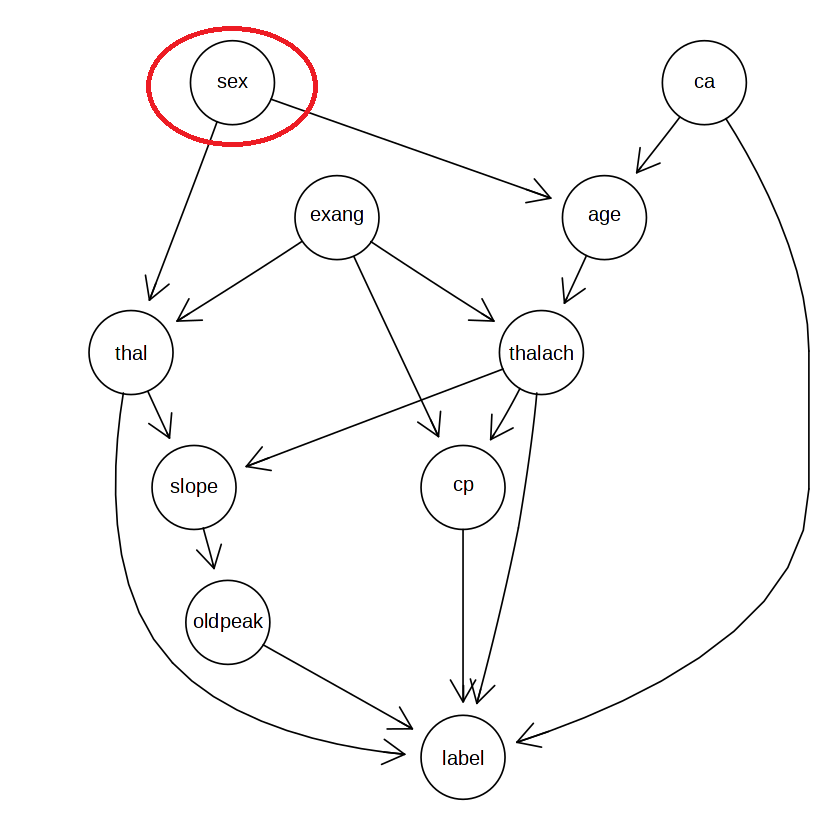}
    \includegraphics[width=0.795\textwidth]{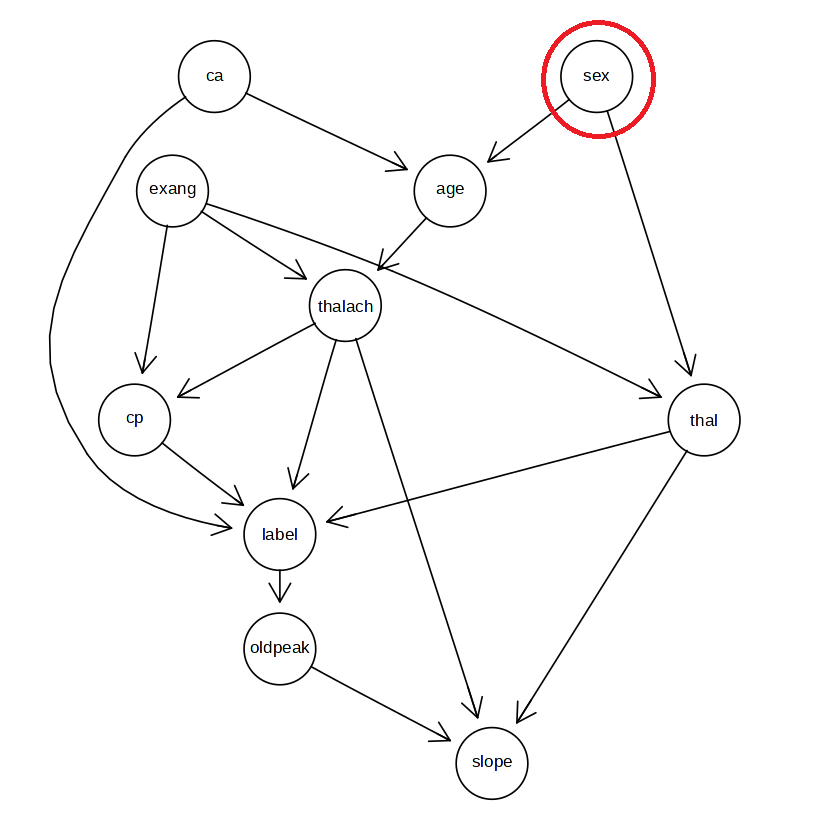}
    \captionsetup{font=small}
    \caption{Heart SelectPercentile.}
    \label{fig:causal-heart-select}
 \end{minipage}
\end{figure*}
